# Supplementary material for: AI Choreographer: Music Conditioned 3D Dance Generation with AIST++
Source: arXiv:2101.08779 source file (2021-07-31)
Supplement: Supplementary file 1 [file genre_correlation_gt.tex]

\begin{figure}[t]
\centering
\includegraphics[width=0.44\textwidth]{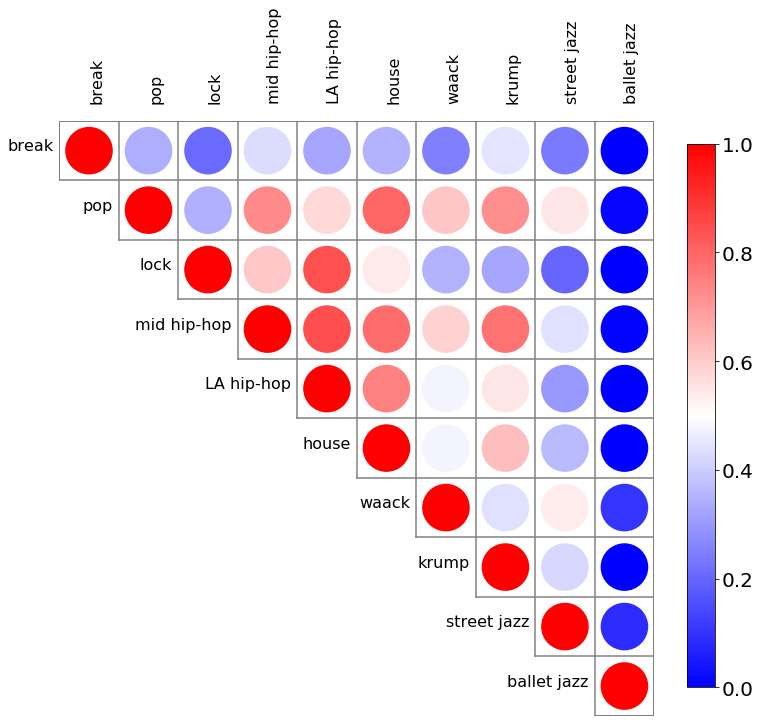}
\caption{\textbf{Motion Similarity in AIST++.} We analyze the similarity between different genres of dance motion in AIST++, which shows distribution difference among genres. For example, ballet jazz is quite different than any other kind of dance.
}
\label{fig:genre_correlation_gt}
\vspace{-3mm}
\end{figure}
