# Supplementary material for: AI Choreographer: Music Conditioned 3D Dance Generation with AIST++
Source: arXiv:2101.08779 source file (2021-07-31)
Supplement: Supplementary file 2 [file genre_correlation_pred.tex]

\begin{figure}[t]
\centering
\includegraphics[width=0.42\textwidth]{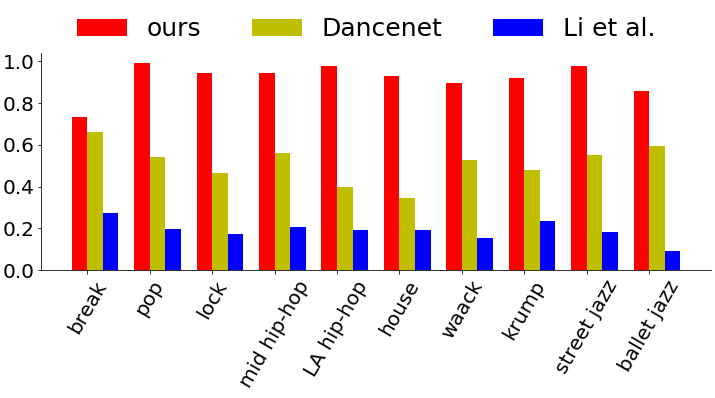}
\caption{\textbf{Genre Consistency between Generated Dance and Music.}
We analyze the genre consistency between the generated dance motion and the input music, of all three methods, on all ten genres. Higher the better.
}
\label{fig:genre_correlation_pred}
\vspace{-3mm}
\end{figure}
