# Supplementary material for: AI Choreographer: Music Conditioned 3D Dance Generation with AIST++
Source: arXiv:2101.08779 source file (2021-07-31)
Supplement: Supplementary file 3 [file user_study_2_years.tex]

\begin{figure*}[t]
\centering
\includegraphics[width=0.8\textwidth]{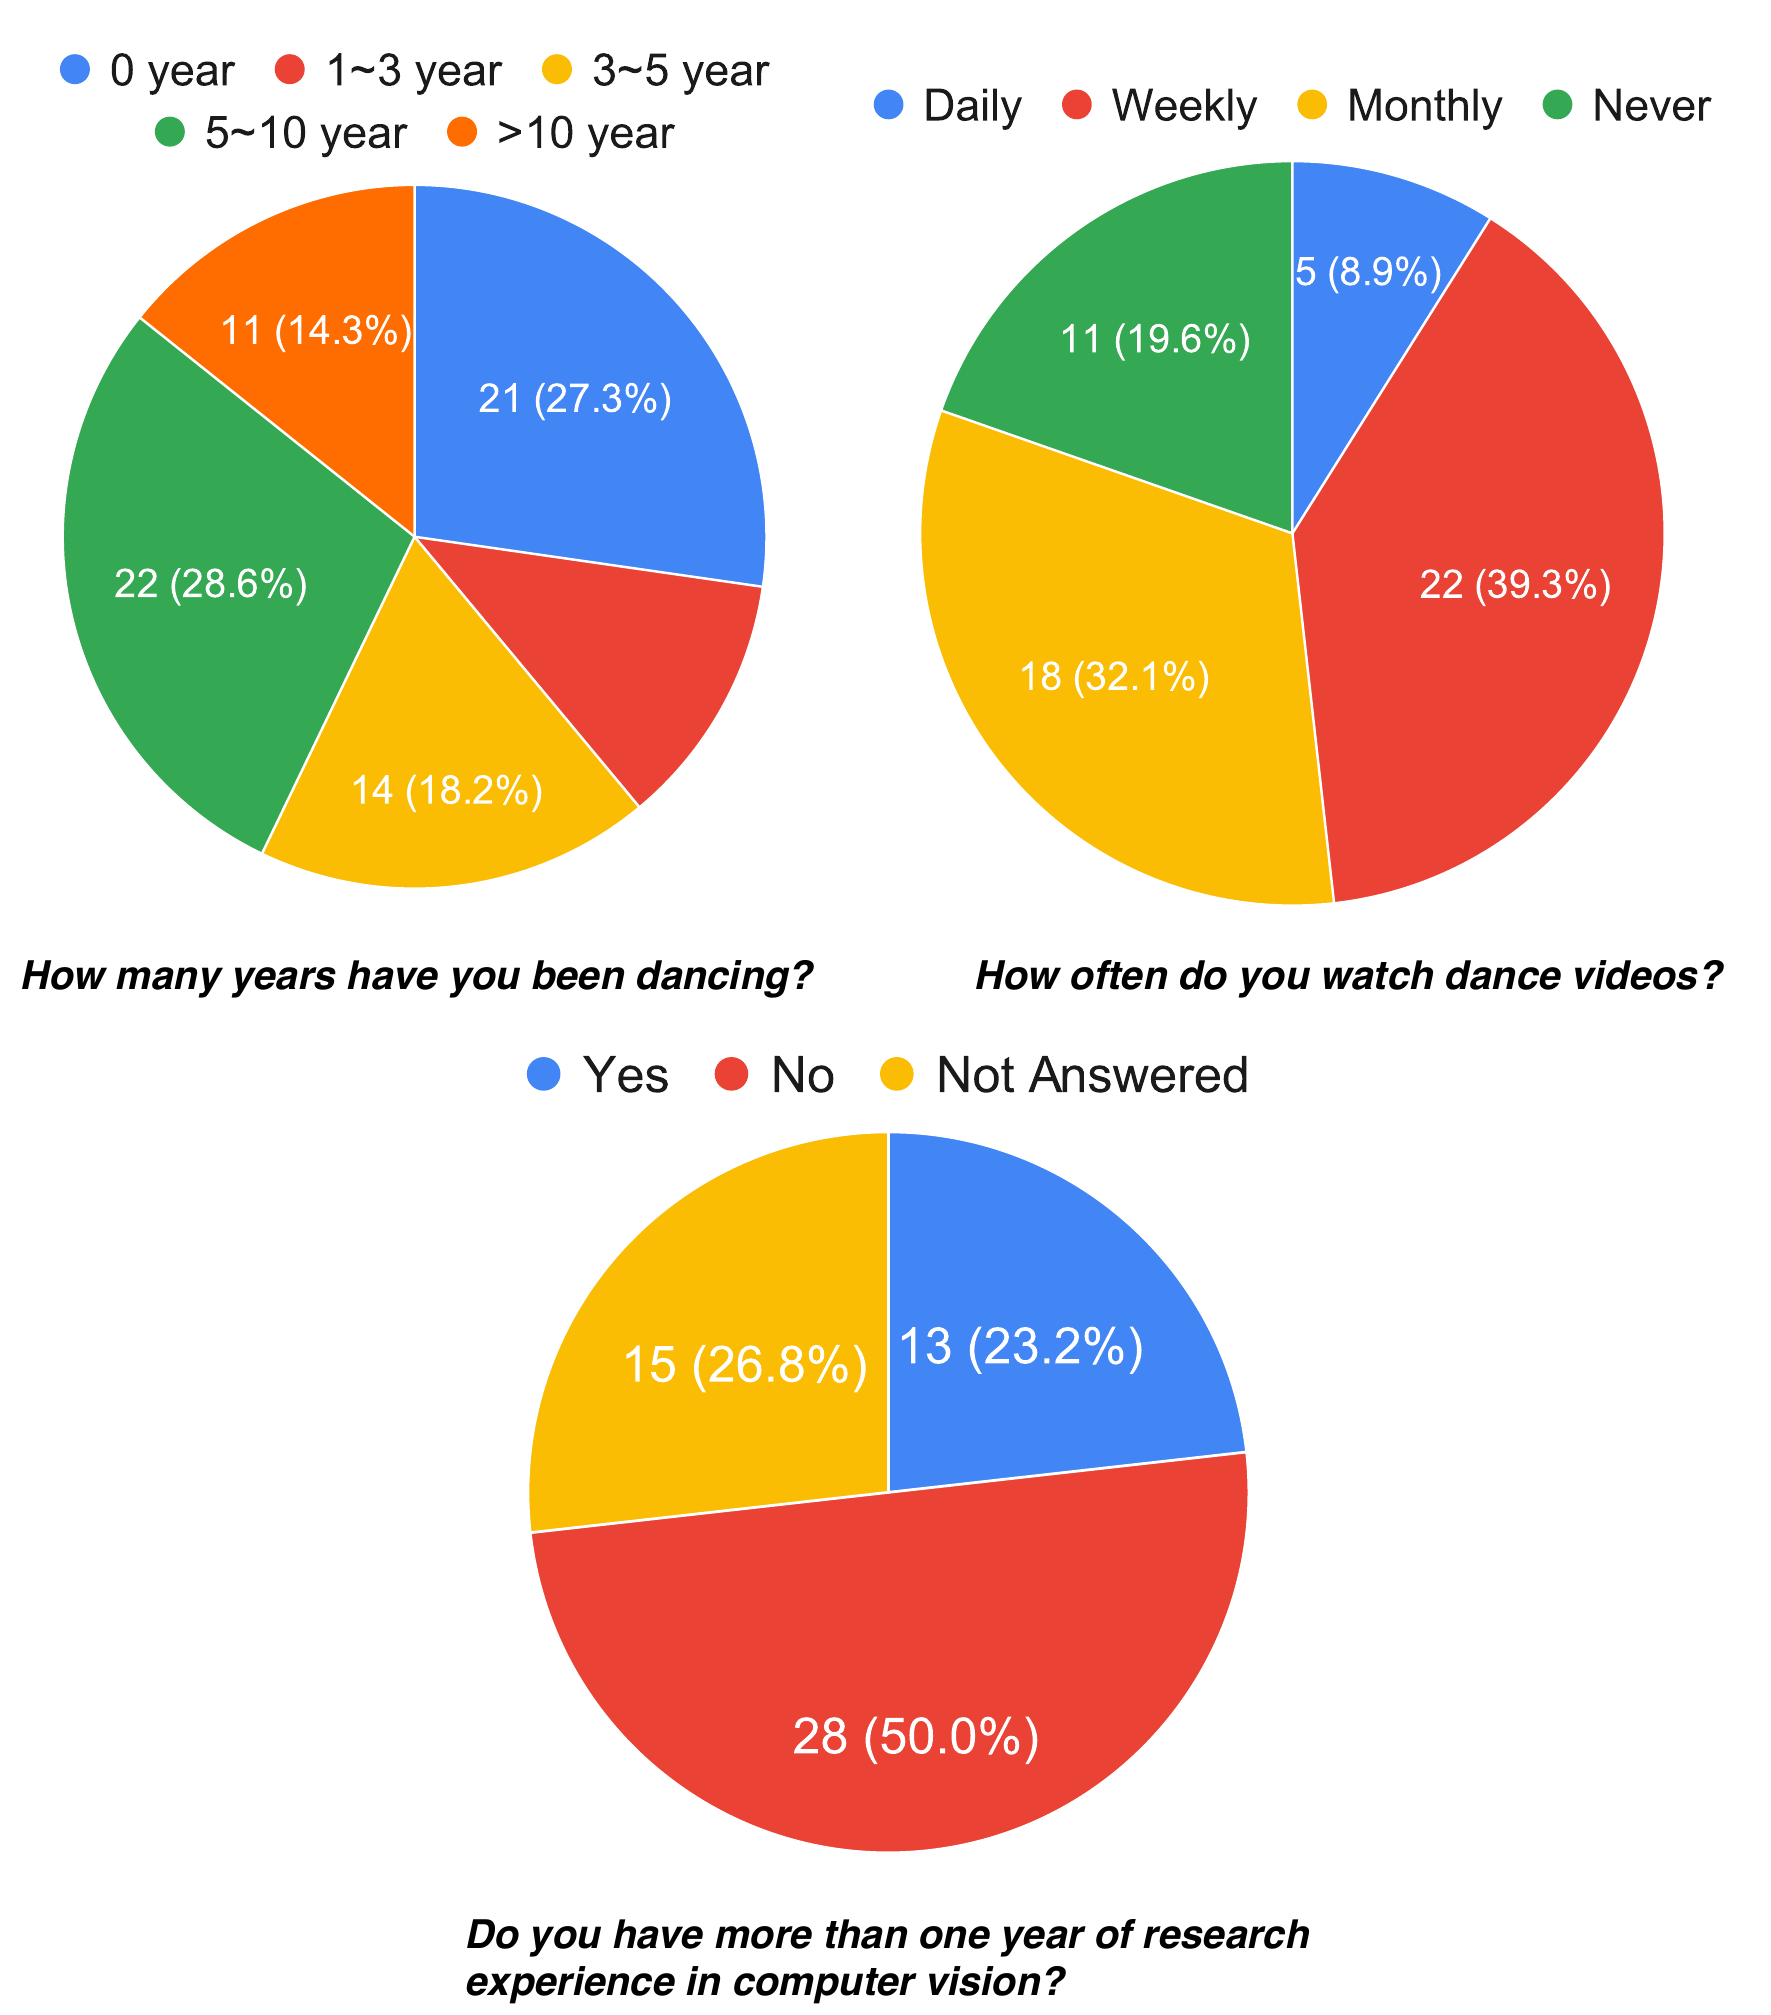}
\caption{\textbf{Participant Demography of the \emph{Realism} User Study.}
}
\label{fig:user_study_2_years}
\vspace{-4mm}
\end{figure*}
